# Supplementary material for: On verifying expectations and observations of intelligent agents
Source: arXiv:2205.00784 source file (2022-05-12)
Supplement: Supplementary file 2 [file supplementary.tex]

%%%% ijcai22.tex

\typeout{IJCAI--22 Instructions for Authors}

% These are the instructions for authors for IJCAI-22.

\documentclass{article}
\pdfpagewidth=8.5in
\pdfpageheight=11in
% The file ijcai22.sty is NOT the same as previous years'
\usepackage{ijcai22}

% Use the postscript times font!
\usepackage{times}
\usepackage{soul}
\usepackage{url}
\usepackage[hidelinks]{hyperref}
\usepackage[utf8]{inputenc}
\usepackage[small]{caption}
\usepackage{graphicx}
\usepackage{amsmath}
\usepackage{amsthm}
\usepackage{thmtools}
\usepackage{thm-restate}
\usepackage{booktabs}
\usepackage{algorithm}
\usepackage{algorithmic}
\urlstyle{same}

\usepackage{todonotes} % added by François to put comments

% the following package is optional:
%\usepackage{latexsym}

% See https://www.overleaf.com/learn/latex/theorems_and_proofs
% for a nice explanation of how to define new theorems, but keep
% in mind that the amsthm package is already included in this
% template and that you must *not* alter the styling.
% \newtheorem{example}{Example}
% \newtheorem{theorem}{Theorem}

% Following comment is from ijcai97-submit.tex:
% The preparation of these files was supported by Schlumberger Palo Alto
% Research, AT\&T Bell Laboratories, and Morgan Kaufmann Publishers.
% Shirley Jowell, of Morgan Kaufmann Publishers, and Peter F.
% Patel-Schneider, of AT\&T Bell Laboratories collaborated on their
% preparation.

% These instructions can be modified and used in other conferences as long
% as credit to the authors and supporting agencies is retained, this notice
% is not changed, and further modification or reuse is not restricted.
% Neither Shirley Jowell nor Peter F. Patel-Schneider can be listed as
% contacts for providing assistance without their prior permission.

% To use for other conferences, change references to files and the
% conference appropriate and use other authors, contacts, publishers, and
% organizations.
% Also change the deadline and address for returning papers and the length and
% page charge instructions.
% Put where the files are available in the appropriate places.

% PDF Info Is REQUIRED.
% Please **do not** include Title and Author information
\pdfinfo{
/TemplateVersion (IJCAI.2022.0)
}

\title{Supplementary materials On the Computational Complexity of Model Checking for Public Observation Logic}

% Single author syntax
% \author{
%     Author Name
%     \affiliations
%     Affiliation
%     \emails
%     pcchair@ijcai-22.org
% }

% Multiple author syntax (remove the single-author syntax above and the \iffalse ... \fi here)
% Check the ijcai22-multiauthor.tex file for detailed instructions
% \iffalse
% \author{
% First Author$^1$
% \and
% Second Author$^2$\and
% Third Author$^{2,3}$\And
% Fourth Author$^4$
% \affiliations
% $^1$First Affiliation\\
% $^2$Second Affiliation\\
% $^3$Third Affiliation\\
% $^4$Fourth Affiliation
% \emails
% \{first, second\}@example.com,
% third@other.example.com,
% fourth@example.com
% }
% \fi

\usepackage{amsmath,amssymb, color, tikz}
\tikzstyle{circNode} = [circle, text centered, draw=black, minimum size= 2em]

 %for automata
 %for application
 %for application

\tikzstyle{world} = [circle, draw, minimum height=9mm]
%%%%added by sujata

\renewcommand{\phi}{\varphi}

%%%% added by Hans

 %math mode is always \it

%\newcommand{\POL}{\mbox{\it POL}}

%\newcommand{\DEL}{\mbox{\it DEL}}

%\newcommand{\PDL}{\mbox{\it PDL}}

%\newcommand{\ETL}{\mbox{\it ETL}}

%\newcommand{\EPL}{\mbox{\it EPL}}
%\newcommand{\EPDL}{\mbox{\it EPDL}}

%\newcommand{\PAL}{\mbox{PAL}}

% \newcommand{\NO}{$\mathsf{FALSE}$ }

\begin{document}

\maketitle

\input{Proofs3Supp}

\input{Proofs5Supp}

\input{Proofs6Supp}

\input{appendix_reductionSAT}
\bibliographystyle{named}
\bibliography{bibliography}
\end{document}
