# Supplementary material for: On verifying expectations and observations of intelligent agents
Source: arXiv:2205.00784 source file (2022-05-12)
Supplement: Supplementary file 3 [file appendix.tex]

\begin{center}
   \Huge{\textbf{Appendix}}
\end{center}

\ 

% \section{Definitions}
% \sujata{In the traffic example, the observation expression $(g^\ast ar^\ast)^\ast$ models the traveller's expectation of traffic signals in case she is in France. In the other one, the observation expression $m$ models the expectation of the receiver in case a decision is made. The size of these observation expressions is defined as follows.} 

%\input{Supplementary/fragmentsdefn}
\input{Supplementary/Proofs3Supp}
\input{Supplementary/Proofs5Supp}
\input{Supplementary/Proofs6Supp}
\input{Supplementary/appendix_reductionSAT} %François has written that
