# Supplementary material for: On verifying expectations and observations of intelligent agents
Source: arXiv:2205.00784 source file (2022-05-12)
Supplement: Supplementary file 8 [file appendix_reductionSAT.tex]

% \section{Efficient  model-checking algorithm for the $\starfree-\existential$ fragment of  $\POL$}
% %Reduction of the existential star-free fragment POL model checking to SAT}
% \label{appendix:starfreeexistentialToSAT}
